# Supplementary material for: The $k$-Fr\'echet distance
Source: arXiv:1903.02353 source file (2019-03-06)

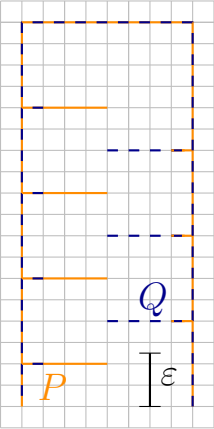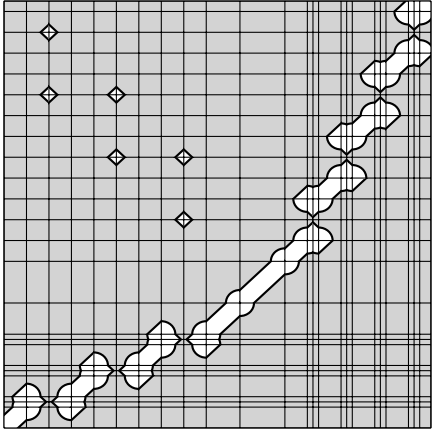

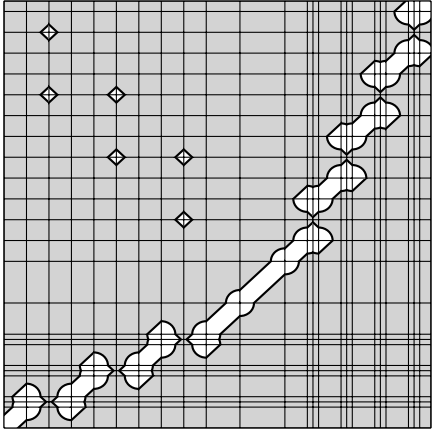

Supplement: Supplementary file 1 [file Wire-appendix.pdf]
